# Supplementary material for: RAPID-RL: A Reconfigurable Architecture with Preemptive-Exits for Efficient Deep-Reinforcement Learning
Source: arXiv:2109.08231 source file (2021-09-16)
Supplement: Supplementary file 1 [file appendix.tex]

\section*{APPENDIX}

\subsection{List of Hyperparamters}
Table ~\ref{app:common}, ~\ref{app:atari} and ~\ref{app:pedra} list the common and task specific hyperparameters used during experiments.
% \aqeel{Any specific reason of grouping the rows of the table \ref{app:common}?}
\begin{table}[h]
\centering
\begin{tabular}{|c|c|p{\textwidth}}
\hline
\textbf{Hyperparameter} & \textbf{Value} \\
\hline
Training Steps (T) & $20 \times 10^6$\\
\hline
Batch Size (B) & 32\\
\hline
Maximum episode length & $108 \times 10^3$\\
\hline
Replay buffer size & $10^5$\\
\hline
Gamma ($\gamma$) & 0.99\\
\hline
Learning start & $80 \times 10^3$\\
\hline
Target Update frequency & $8 \times 10^3$\\
\hline
Learning Rate & $6.25 \times 10^5$\\
\hline
Adam Epsilon ($\epsilon$) & $1.5 \times 10^-4$\\
\hline
Train interval & $4$\\
\hline
Validation Episodes & $20$\\
\hline
Validation interval & $1 \times 10^6$\\
\hline
Validation Memory Size  & $20 \times 10^3$\\
\hline
Priority weight & $0.4$\\
\hline
Priority exponent & $0.5$\\
\hline
Multi-step learning parameter & $3$\\
\hline
Number of atoms & $51$\\
\hline
Noisy net Std ($\sigma_0$) & $0.5$\\
\hline
Confidence threshold (C) & $0.8$\\
\hline
Preemptive threshold (P) & $0.7$\\
\hline
\end{tabular}
\vspace{2mm}
\caption{Common hyperparameters.}
%\vspace{-4mm}
\label{app:common}
\end{table}

\begin{table}[h]
\centering
\begin{tabular}{|c|c|p{\textwidth}}
\hline
\textbf{Hyperparameter} & \textbf{Value} \\
\hline
Input size & $4 \times 84 \times 84$\\
\hline
Noisy net $V_{min}$ & $-10$\\
\hline
Noisy net $V_{max}$ & $10$\\
\hline
\end{tabular}
\vspace{2mm}
\caption{Specific hyperparameters for Atari 2600 task.}
%\vspace{-4mm}
\label{app:atari}
\end{table}

\begin{table}[h]
\centering
\begin{tabular}{|c|c|p{\textwidth}}
\hline
\textbf{Hyperparameter} & \textbf{Value} \\
\hline
Input size & $3 \times 103 \times 103$\\
\hline
Number of actions & $25$\\
\hline
Switch env steps & $50 \times 10^3$\\
\hline
Crash threshold & 1.3 \\
\hline
Noisy net $V_{min}$ & $-1$\\
\hline
Noisy net $V_{max}$ & $1$\\
\hline
\end{tabular}
\vspace{2mm}
\caption{Specific hyperparameters for Drone navigation task.}
%\vspace{-4mm}
\label{app:pedra}
\end{table}
